# Supplementary material for: Topological invariant of non-Hermitian space-time modulated photonic crystals
Source: arXiv:2412.20636 source file (2024-12-30)
Supplement: Supplementary file 1 [file Supp.pdf]

# Supplemental Material:
# Topological invariant of non-Hermitian space-time modulated photonic crystals

Xiaoke Gao [1] Xiaoyu Zhao [1] Jiawei Wang [1] Xikui Ma [1] and Tianyu Dong [1,*]
[1] *School of Electrical Engineering, Xi'an Jiaotong University, Xi'an 710049, China.*
(Dated: December 29, 2024)

## S1. TRANSFER/SCATTERING MATRIX METHOD FOR STMPCS

We consider a space-time-modulated photonic crystal (STMPC) that consists of dielectrics and photonic time crystals (PTCs) arranged regularly in space, which are indicated by $\varepsilon_{\text{diel}}$ and $\varepsilon^{\text{PTC}}(t)$, respectively, as illustrated in FIG. S1**a**. The thickness of a unit is $d = d_{\text{m}} + d_{\text{t}}$, with the thicknesses of the dielectric and PTC layers being $d_{\text{m}}$ and $d_{\text{t}}$, respectively. In our analysis, we consider the polarization mode of $\{E_x, H_y, k_z\}$, as illustrated in FIG. S1**a**. Next, by identifying the propagation modes of electromagnetic waves inside each layer of the medium, as well as the transfer and/or scattering equations at material boundaries, we can formulate the transfer/scattering cascading approach to handle multilayer STMPCs composed of PTCs and dielectrics.

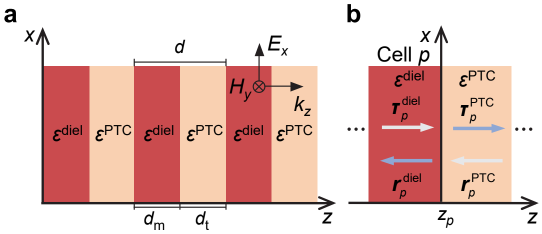


FIG. S1. **Illustration of a space-time-modulated photonic crystal (STMPC). a**, Multi-layers consisted of dielectrics and PTCs. **b**, $p$-th interface between dielectrics and PTCs.

### A. Fundamental solutions in PTCs and dielectrics

The governing equation for the parallel polarized electromagnetic waves $E_x^{\text{PTC}}(z,t)$ inside free-source PTCs reads,

$$\nabla^2 E_x^{\text{PTC}}(z,t) - \mu_0 \partial_t^2 \left[\varepsilon^{\text{PTC}}(t) E_x^{\text{PTC}}(z,t)\right] = 0. \tag{S1}$$

Here, the subscript $x$ denotes the polarized direction of the electric field. By considering the temporal periodicity of the PTC, *i.e.*, $\varepsilon^{\text{PTC}}(t+T) = \varepsilon^{\text{PTC}}(t)$, where $T$ denotes the temporal period, the solution to the (S1) can be expressed as

$$E_x^{\text{PTC}}(z,t) = \sum_{n=-\infty}^{\infty} E_{x,n}^{\text{PTC}} e^{\mathrm{i}[qz-(\omega+n\Omega)t]}, \tag{S2}$$

with the wave number $q$ and Bloch quasi-frequency $\omega$ according to the Floquet-Bloch theorem, where $\Omega = 2\pi/T$ and $n$ denotes the order of time harmonics. The time-varying permittivity can be expand as a Fourier series, namely, $\varepsilon_t(t) = \sum_m \varepsilon_m^{\text{PTC}} e^{-\mathrm{i}(\omega+m\Omega)t}$, where $s$ denotes the order of harmonic factors. Insert the series expansions of $E_x^{\text{PTC}}(z,t)$ and $\varepsilon^{\text{PTC}}(t)$ into (S1), we can obtain

$$q^2 \sum_{n=-\infty}^{\infty} E_{x,n}^{\text{PTC}} e^{\mathrm{i}[qz-(\omega+n\Omega)t]} = \mu_0 \sum_{n=-\infty}^{\infty} \sum_{m=-\infty}^{\infty} \left[\omega+(n+m)\Omega\right]^2 \varepsilon_m^{\text{PTC}} E_{x,n}^{\text{PTC}} e^{\mathrm{i}\{qz-[\omega+(n+m)\Omega]t\}}. \tag{S3}$$

By changing the summation index of the series on the right-hand side of (S3), *i.e.*, $n \to n-s$, (S3) can be further re-written as

$$q^2 \sum_{n=-\infty}^{\infty} E_{x,n}^{\text{PTC}} e^{\mathrm{i}[qz-(\omega+n\Omega)t]} = \mu_0 \sum_{n=-\infty}^{\infty} \sum_{m=-\infty}^{\infty} (\omega+n\Omega)^2 \varepsilon_m^{\text{PTC}} E_{x,n-m}^{\text{PTC}} e^{\mathrm{i}[qz-(\omega+n\Omega)t]}. \tag{S4}$$

* Corresponding author. Email: tydong@mail.xjtu.edu.cn

Now, by considering the orthogonality of harmonic functions, (S4) can be simplified to

$$q^2 E_{x,n}^{\mathrm{PTC}} = \mu_0 \sum_{m=-\infty}^{\infty} (\omega + n\Omega)^2 \varepsilon_m^{\mathrm{PTC}} E_{x,n-m}^{\mathrm{PTC}} \tag{S5}$$

for each harmonic mode number $n \in \mathbb{Z}$. By exchanging the summation indices of $\varepsilon_m^{\mathrm{PTC}}$ and $E_{x,n-m}^{\mathrm{PTC}}$ on the right-hand side of (S5), we arrive at

$$q^2 E_{x,n}^{\mathrm{PTC}} = \sum_{m=-\infty}^{\infty} \left(\frac{\omega + n\Omega}{c_0}\right)^2 \varepsilon_{n-m}^{\mathrm{PTC}} E_{x,m}^{\mathrm{PTC}}, \quad n \in \mathbb{Z}, \tag{S6}$$

which can be expressed in a compact matrix form as Truncate $s$ and $m$ both from $-N$ to $N$. The matrix form of (S6) reads

$$(\mathcal{D} \cdot \mathcal{E})\psi = q^2 \psi. \tag{S7}$$

In practice, the infinite series are often truncated within a limited range of $[-N, N]$. In this regards, we have $\mathcal{D} = \mu_0 \mathrm{diag}[(\omega - N\Omega)^2, \ldots, \omega^2, \ldots, (\omega + N\Omega)^2]$ being a diagonal matrix; $\psi = \left(E_{x,-N}^{\mathrm{PTC}}, E_{x,-N+1}^{\mathrm{PTC}}, \ldots, E_{x,0}^{\mathrm{PTC}}, \ldots, E_{x,N-1}^{\mathrm{PTC}}, E_{x,N}^{\mathrm{PTC}}\right)^{\mathrm{T}}$; $\mathcal{E}$ is the matrix that reflects the material information, which reads

$$\mathcal{E} = \begin{pmatrix} \varepsilon_0^{\mathrm{PTC}} & \varepsilon_{-1}^{\mathrm{PTC}} & \cdots & \varepsilon_{-2N}^{\mathrm{PTC}} \\ \varepsilon_1^{\mathrm{PTC}} & \varepsilon_0^{\mathrm{PTC}} & \cdots & \varepsilon_{-2N+1}^{\mathrm{PTC}} \\ \vdots & \vdots & \ddots & \vdots \\ \varepsilon_{2N}^{\mathrm{PTC}} & \varepsilon_{2N-1}^{\mathrm{PTC}} & \cdots & \varepsilon_0^{\mathrm{PTC}} \end{pmatrix}. \tag{S8}$$

Therefore, the wave number $q^2$ can be obtained by solving the eigenvalue problem described in (S7). Now, the electromagnetic wave in the PTC can be expressed as

$$E_x^{\mathrm{PTC}}(z,t) = \sum_{n=-N}^{N} \sum_{l=1}^{2N+1} \psi_{l,n} e^{-\mathrm{i}(\omega+n\Omega)t} \left(\tau_l^{\mathrm{PTC}} e^{\mathrm{i}q_l z} + r_l^{\mathrm{PTC}} e^{-\mathrm{i}q_l z}\right), \tag{S9a}$$

$$H_y^{\mathrm{PTC}}(z,t) = \sum_{n=-N}^{N} \sum_{l=1}^{2N+1} \frac{q_l \psi_{l,n}}{\omega + n\Omega} e^{-\mathrm{i}(\omega+n\Omega)t} \left(\tau_l^{\mathrm{PTC}} e^{\mathrm{i}q_l z} - r_l^{\mathrm{PTC}} e^{-\mathrm{i}q_l z}\right), \tag{S9b}$$

where $q_l^2$ is denoted as the $l$-th eigenvalue, and $\psi_l$ denotes the corresponding normalized eigenvector with components $\psi_{l,n} = E_{x,l,n}^{\mathrm{PTC}}$; in addition, the coefficients $\tau_l^{\mathrm{PTC}}$ and $r_l^{\mathrm{PTC}}$ are the mode amplitudes of the forward and backward waves with wave number of $q_l$ inside the PTCs, respectively, which can be determined by matching the boundary conditions.

Similarly, in the dielectric $\varepsilon^{\mathrm{diel}}$, the $p$-polarized electromagnetic waves with frequencies of $\omega + n\Omega$ ($n \in [-N, N]$) read

$$E_x^{\mathrm{diel}}(z,t) = \sum_{n=-N}^{N} e^{-\mathrm{i}(\omega+n\Omega)t} \left(\tau_n^{\mathrm{diel}} e^{\mathrm{i}k_n^{\mathrm{diel}} z} + r_n^{\mathrm{diel}} e^{-\mathrm{i}k_n^{\mathrm{diel}} z}\right), \tag{S10a}$$

$$H_y^{\mathrm{diel}}(z,t) = \sum_{n=-N}^{N} \frac{k_n^{\mathrm{diel}}}{\omega + n\Omega} e^{-\mathrm{i}(\omega+n\Omega)t} \left(\tau_n^{\mathrm{diel}} e^{\mathrm{i}k_n^{\mathrm{diel}} z} - r_n^{\mathrm{diel}} e^{-\mathrm{i}k_n^{\mathrm{diel}} z}\right). \tag{S10b}$$

where the coefficients $\tau_n^{\mathrm{diel}}$ and $r_n^{\mathrm{diel}}$ denote the amplitudes of the forward and backward harmonics inside the dielectrics with frequency of $\omega + n\Omega$ and wave number $k_{m,n}$, which can be determined by matching the boundary conditions.

### B. Scattering matrix at dielectric–PTC interface

Next, we consider an interface of a dielectric and a PTC located at $z = z_p$, as shown in FIG. S1**b**. The electromagnetic wave in the $p$-th cell reads

$$E_{x,p}^{\mathrm{PTC}}(z,t) = \sum_{n=-N}^{N} \sum_{l=1}^{2N+1} \psi_{l,n} e^{-\mathrm{i}(\omega+n\Omega)t} \left(\tau_{p,l}^{\mathrm{PTC}} e^{\mathrm{i}q_l z} + r_{p,l}^{\mathrm{PTC}} e^{-\mathrm{i}q_l z}\right), \tag{S11a}$$

$$H_{y,p}^{\rm PTC}(z,t)=\sum_{n=-N}^{N}\sum_{l=1}^{2N+1}\frac{q_l\psi_{l,n}}{\omega+n\Omega}e^{-{\rm i}(\omega+n\Omega)t}\left(\tau_{p,l}^{\rm PTC}e^{{\rm i}q_l z}-r_{p,l}^{\rm PTC}e^{-{\rm i}q_l z}\right) \tag{S11b}$$

for PTCs when $z_p-d_{\rm m}\le z\le z_p$ and

$$E_{x,p}^{\rm diel}(z,t)=\sum_{n=-N}^{N}e^{-{\rm i}(\omega+n\Omega)t}\left(\tau_{p,n}^{\rm diel}e^{{\rm i}k_n^{\rm diel}z}+r_{p,n}^{\rm diel}e^{-{\rm i}k_n^{\rm diel}z}\right), \tag{S11c}$$

$$H_{y,p}^{\rm diel}(z,t)=\sum_{n=-N}^{N}\frac{k_n^{\rm diel}}{\omega+n\Omega}e^{-{\rm i}(\omega+n\Omega)t}\left(\tau_{p,n}^{\rm diel}e^{{\rm i}k_n^{\rm diel}z}-r_{p,n}^{\rm diel}e^{-{\rm i}k_n^{\rm diel}z}\right) \tag{S11d}$$

for dielectric when $z_p\le z\le z_p+d_{\rm t}$, where $\tau_{p,l}^{\rm PTC}$ (or $r_{p,l}^{\rm PTC}$ denotes the coefficients of the forward (or backward) waves with wave number $q_l$ in PTC layer of the $p$-th cell; $\tau_{p,n}^{\rm diel}$ (or $r_{p,n}^{\rm diel}$) denotes the coefficients of the forward (or backward) waves with frequency of $\omega+n\Omega$ in dielectric layer of the $p$-th cell.

At the boundary $z=z_p$, the tangential components of the electric fields and magnetic fields are respectively continuous at every moment, namely,

$$E_{x,p}^{\rm PTC}(z_p,t)=E_{x,p}^{\rm diel}(z_p,t), \tag{S12a}$$

$$H_{y,p}^{\rm PTC}(z_p,t)=H_{y,p}^{\rm diel}(z_p,t),\qquad \forall t. \tag{S12b}$$

By considering the orthogonality of complex exponential functions $e^{-{\rm i}(\omega+n\Omega)t}$ within $n\in[-N,N]$, (S12a) and (S12b) can be further expressed respectively as

$$\sum_{l=1}^{2N+1}\psi_{l,n}\left(\tau_{p,l}^{\rm PTC}e^{{\rm i}q_l z_p}+r_{p,l}^{\rm PTC}e^{-{\rm i}q_l z_p}\right)=\tau_{p,n}^{\rm diel}e^{{\rm i}k_n^{\rm diel}z_p}+r_{p,n}^{\rm diel}e^{-{\rm i}k_n^{\rm diel}z_p}, \tag{S13a}$$

$$\sum_{l=1}^{2N+1}\frac{q_l\psi_{l,n}}{\omega+n\Omega}\left(\tau_{p,l}^{\rm PTC}e^{{\rm i}q_l z_p}-r_{p,l}^{\rm PTC}e^{-{\rm i}q_l z_p}\right)=\frac{k_n^{\rm diel}}{\omega+n\Omega}\left(\tau_{p,n}^{\rm diel}e^{{\rm i}k_n^{\rm diel}z_p}-r_{p,n}^{\rm diel}e^{-{\rm i}k_n^{\rm diel}z_p}\right) \tag{S13b}$$

for each $n\in[-N,N]$, which can be rewritten in a matrix form as

$$\Psi\boldsymbol{\phi}_p^{\rm PTC}\boldsymbol{\tau}_p^{\rm PTC}-\boldsymbol{\phi}_p^{*\rm diel}\boldsymbol{r}_p^{\rm diel}=\boldsymbol{\phi}_p^{\rm diel}\boldsymbol{\tau}_p^{\rm diel}-\Psi\boldsymbol{\phi}_p^{*\rm PTC}\boldsymbol{r}_p^{\rm PTC}, \tag{S14a}$$

$$\Psi\mathcal{Q}\boldsymbol{\phi}_p^{\rm PTC}\boldsymbol{\tau}_p^{\rm PTC}+\mathcal{K}\boldsymbol{\phi}_p^{*\rm diel}\boldsymbol{r}_p^{\rm diel}=\mathcal{K}\boldsymbol{\phi}_p^{\rm diel}\boldsymbol{\tau}_p^{\rm diel}+\Psi\mathcal{Q}\boldsymbol{\phi}_{t,p}^{*\rm PTC}\boldsymbol{r}_p^{\rm PTC}, \tag{S14b}$$

and

$$\begin{pmatrix}\Psi\boldsymbol{\phi}_p^{\rm PTC} & -\boldsymbol{\phi}_{m,p}^{*\rm diel}\\ \Psi\mathcal{Q}\boldsymbol{\phi}_p^{\rm PTC} & \mathcal{K}\boldsymbol{\phi}_p^{*\rm diel}\end{pmatrix}\cdot\begin{pmatrix}\boldsymbol{\tau}_p^{\rm PTC}\\ \boldsymbol{r}_p^{\rm diel}\end{pmatrix}=\begin{pmatrix}\boldsymbol{\phi}_p^{\rm diel} & -\Psi\boldsymbol{\phi}_p^{*\rm PTC}\\ \mathcal{K}\boldsymbol{\phi}_p^{\rm diel} & \Psi\mathcal{Q}\boldsymbol{\phi}_p^{*\rm PTC}\end{pmatrix}\cdot\begin{pmatrix}\boldsymbol{\tau}_p^{\rm diel}\\ \boldsymbol{r}_p^{\rm PTC}\end{pmatrix}, \tag{S14c}$$

where

$$\boldsymbol{\tau}_p^{\rm diel}=[\tau_{p,-N}^{\rm diel},\dots,\tau_{p,0}^{\rm diel},\dots,\tau_{p,N}^{\rm diel}]^{\rm T}, \tag{S15a}$$

$$\boldsymbol{r}_p^{\rm diel}=[r_{p,-N}^{\rm diel},\dots,r_{p,0}^{\rm diel},\dots,r_{p,N}^{\rm diel}]^{\rm T}, \tag{S15b}$$

$$\boldsymbol{\tau}_p^{\rm PTC}=[\tau_{p,0}^{\rm PTC},\dots,\tau_{p,N}^{\rm PTC},\dots,\tau_{p,2N+1}^{\rm PTC}]^{\rm T}, \tag{S15c}$$

$$\boldsymbol{r}_p^{\rm PTC}=[r_{p,0}^{\rm PTC},\dots,r_{p,N}^{\rm PTC},\dots,r_{p,2N+1}^{\rm PTC}]^{\rm T}, \tag{S15d}$$

$$\Psi=[\psi_1,\dots,\psi_{N+1},\dots,\psi_{2N+1}], \tag{S15e}$$

$$\mathcal{Q}={\rm diag}[q_1,\dots,q_{N+1},\dots,q_{2N+1}], \tag{S15f}$$

$$\mathcal{K}={\rm diag}[k_{-N}^{\rm diel},\dots,k_0^{\rm diel},\dots,k_N^{\rm diel}], \tag{S15g}$$

$$\boldsymbol{\phi}_p^{\rm PTC}={\rm diag}[e^{{\rm i}q_1 z_p},\dots,e^{{\rm i}q_{N+1}z_p},\dots,e^{{\rm i}q_{2N+1}z_p}], \tag{S15h}$$

$$\boldsymbol{\phi}_p^{\rm diel}={\rm diag}[e^{{\rm i}k_{-N}^{\rm diel}z_p},\dots,e^{{\rm i}k_0^{\rm diel}z_p},\dots,e^{{\rm i}k_N^{\rm diel}z_p}]. \tag{S15i}$$

### C. Cascading scattering matrices

Now, we can handle layered problems by matching the boundary conditions at interfaces. For the $p$-th and $p+1$-th cells inside a multilayered structure, as shown in FIG. S2, the boundary equations at the interfaces $z=z_{p,1}$ and $z=z_{p,2}$ can be written in block matrix form as

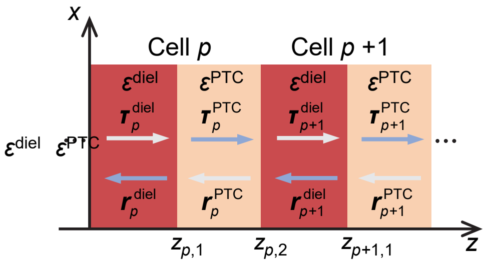


FIG. S2. Two cells of a multilayer structure.

$$\begin{pmatrix} \Psi & -\mathbb{I} \\ \Psi\mathcal{Q} & \mathcal{K} \end{pmatrix} \cdot \begin{pmatrix} \boldsymbol{\phi}_{p,1}^{\mathrm{PTC}} & 0 \\ 0 & \boldsymbol{\phi}_{p,1}^{*\mathrm{diel}} \end{pmatrix} \cdot \begin{pmatrix} \boldsymbol{\tau}_p^{\mathrm{PTC}} \\ \boldsymbol{r}_p^{\mathrm{diel}} \end{pmatrix} = \begin{pmatrix} \mathbb{I} & -\Psi \\ \mathcal{K} & \Psi\mathcal{Q} \end{pmatrix} \cdot \begin{pmatrix} \boldsymbol{\phi}_{p,1}^{\mathrm{diel}} & 0 \\ 0 & \boldsymbol{\phi}_{p,1}^{*\mathrm{PTC}} \end{pmatrix} \cdot \begin{pmatrix} \boldsymbol{\tau}_p^{\mathrm{diel}} \\ \boldsymbol{r}_p^{\mathrm{PTC}} \end{pmatrix}, \tag{S16a}$$

$$\begin{pmatrix} \mathbb{I} & -\Psi \\ \mathcal{K} & \Psi\mathcal{Q} \end{pmatrix} \cdot \begin{pmatrix} \boldsymbol{\phi}_{p,2}^{\mathrm{diel}} & 0 \\ 0 & \boldsymbol{\phi}_{p,2}^{*\mathrm{PTC}} \end{pmatrix} \cdot \begin{pmatrix} \boldsymbol{\tau}_{p+1}^{\mathrm{diel}} \\ \boldsymbol{r}_p^{\mathrm{PTC}} \end{pmatrix} = \begin{pmatrix} \Psi & -\mathbb{I} \\ \Psi\mathcal{Q} & \mathcal{K} \end{pmatrix} \cdot \begin{pmatrix} \boldsymbol{\phi}_{p,2}^{\mathrm{PTC}} & 0 \\ 0 & \boldsymbol{\phi}_{p,2}^{*\mathrm{diel}} \end{pmatrix} \cdot \begin{pmatrix} \boldsymbol{\tau}_p^{\mathrm{PTC}} \\ \boldsymbol{r}_{p+1}^{\mathrm{diel}} \end{pmatrix}, \tag{S16b}$$

where the phases matrices $\boldsymbol{\phi}_p$ read

$$\boldsymbol{\phi}_{p,1}^{\mathrm{PTC}} = \mathrm{diag}[e^{-\mathrm{i}q_1 d_{\mathrm{t}}/2}, \dots, e^{-\mathrm{i}q_{N+1} d_{\mathrm{t}}/2}, \dots, e^{-\mathrm{i}q_{2N+1} d_{\mathrm{t}}/2}], \tag{S17a}$$

$$\boldsymbol{\phi}_{p,1}^{\mathrm{diel}} = \mathrm{diag}[e^{\mathrm{i}k_{-N}^{\mathrm{diel}} d_{\mathrm{m}}/2}, \dots, e^{\mathrm{i}k_0^{\mathrm{diel}} d_{\mathrm{m}}/2}, \dots, e^{\mathrm{i}k_N^{\mathrm{diel}} d_{\mathrm{m}}/2}], \tag{S17b}$$

to avoid the numerical problems caused by the complex wave vectors. In addition, $\boldsymbol{\phi}_{p,2}^{\mathrm{PTC}} = \boldsymbol{\phi}_{p,1}^{*\mathrm{PTC}}$ and $\boldsymbol{\phi}_{p,2}^{\mathrm{diel}} = \boldsymbol{\phi}_{p,1}^{*\mathrm{diel}}$. In (S16a) and (S16b), the coefficients $\boldsymbol{\tau}$'s and $\boldsymbol{r}$'s correspond to the forward and backward waves with origin set at the center of each layers, respectively. In a more compact form, (S16a) and (S16b) can be re-written as

$$\mathcal{T} \cdot \Phi_{p,1}^{\mathrm{Pd}} \cdot \mathcal{C}_{p,p}^{\mathrm{Pd}} = \mathcal{M} \cdot \Phi_{p,1}^{\mathrm{dP}} \cdot \mathcal{C}_{p,p}^{\mathrm{dP}}, \tag{S18a}$$

$$\mathcal{M} \cdot \Phi_{p,2}^{\mathrm{dP}} \cdot \mathcal{C}_{p+1,p}^{\mathrm{dP}} = \mathcal{T} \cdot \Phi_{p,2}^{\mathrm{Pd}} \cdot \mathcal{C}_{p,p+1}^{\mathrm{Pd}}, \tag{S18b}$$

where

$$\mathcal{T} = \begin{pmatrix} \Psi & -\mathbb{I} \\ \Psi\mathcal{Q} & \mathcal{K} \end{pmatrix}. \tag{S19a}$$

$$\mathcal{M} = \begin{pmatrix} \mathbb{I} & -\Psi \\ \mathcal{K} & \Psi\mathcal{Q} \end{pmatrix}, \tag{S19b}$$

$$\Phi_{p,1(2)}^{\mathrm{Pd}} = \mathrm{diag}[\boldsymbol{\phi}_{p,1(2)}^{\mathrm{PTC}}, \boldsymbol{\phi}_{p,1(2)}^{*\mathrm{diel}}], \tag{S19c}$$

$$\Phi_{p,1(2)}^{\mathrm{dP}} = \mathrm{diag}[\boldsymbol{\phi}_{p,1(2)}^{\mathrm{diel}}, \boldsymbol{\phi}_{p,1(2)}^{*\mathrm{PTC}}], \tag{S19d}$$

$$\mathcal{C}_{p,p+1}^{\mathrm{Pd}} = [\boldsymbol{\tau}_p^{\mathrm{PTC}}, \boldsymbol{r}_{p+1}^{\mathrm{diel}}]^{\mathrm{T}}, \tag{S19e}$$

$$\mathcal{C}_{p,p}^{\mathrm{Pd}} = [\boldsymbol{\tau}_p^{\mathrm{PTC}}, \boldsymbol{r}_p^{\mathrm{diel}}]^{\mathrm{T}}, \tag{S19f}$$

$$\mathcal{C}_{p,p}^{\mathrm{dP}} = [\boldsymbol{\tau}_p^{\mathrm{diel}}, \boldsymbol{r}_p^{\mathrm{PTC}}]^{\mathrm{T}}, \tag{S19g}$$

$$\mathcal{C}_{p+1,p}^{\mathrm{dP}} = [\boldsymbol{\tau}_{p+1}^{\mathrm{diel}}, \boldsymbol{r}_p^{\mathrm{PTC}}]^{\mathrm{T}}. \tag{S19h}$$

We can write the boundary equations (S16a) and (S16b) in the context of scattering matrices, which read

$$\mathcal{C}_{p,p}^{\mathrm{Pd}} = \mathcal{S}_{(\mathrm{diel},p)\to(\mathrm{PTC},p)} \cdot \mathcal{C}_{p,p}^{\mathrm{dP}}, \tag{S20a}$$

$$\mathcal{C}_{p+1,p}^{\mathrm{dP}} = \mathcal{S}_{(\mathrm{PTC},p)\to(\mathrm{diel},p+1)} \cdot \mathcal{C}_{p,p+1}^{\mathrm{Pd}}, \tag{S20b}$$

where the generalized scattering matrix $\mathcal{S}_{(\mathrm{diel},p)\to(\mathrm{PTC},p)}$ and $\mathcal{S}_{(\mathrm{PTC},p)\to(\mathrm{diel},p+1)}$ can be derived from (S20a) and (S20a), respectively reading as

$$\mathcal{S}_{(\mathrm{diel},p)\to(\mathrm{PTC},p)} = (\Phi_{p,1}^{\mathrm{Pd}})^{-1} \cdot \mathcal{T}^{-1} \cdot \mathcal{M} \cdot \Phi_{p,1}^{\mathrm{dP}} \tag{S21a}$$

$$\mathcal{S}_{(\mathrm{PTC},p)\to(\mathrm{diel},p+1)} = (\Phi_{p,2}^{\mathrm{dP}})^{-1} \cdot \mathcal{M}^{-1} \mathcal{T} \cdot \Phi_{p,2}^{\mathrm{Pd}}. \tag{S21b}$$

Now, (S20a) and (S20b) can be cascaded and form a new scattering systems as

$$\mathcal{C}^{\text{dd}}_{p+1,p} = \mathcal{S}_{(\text{diel},p)\to(\text{diel},p+1)} \cdot \mathcal{C}^{\text{dd}}_{p,p+1}, \tag{S22}$$

where the elements of $\mathcal{S}_{(\text{diel},p)\to(\text{diel},p+1)}$ reads

$$\mathcal{S}^{11}_{(\text{diel},p)\to(\text{diel},p+1)} = \mathcal{S}^{11}_{(\text{PTC},p)\to(\text{diel},p+1)} \cdot \chi_1 \cdot \mathcal{S}^{11}_{(\text{diel},p)\to(\text{PTC},p)}, \tag{S23a}$$

$$\mathcal{S}^{12}_{(\text{diel},p)\to(\text{diel},p+1)} = \mathcal{S}^{12}_{(\text{PTC},p)\to(\text{diel},p+1)} + \mathcal{S}^{11}_{(\text{PTC},p)\to(\text{diel},p+1)} \cdot \chi_1 \cdot \mathcal{S}^{12}_{(\text{diel},p)\to(\text{PTC},p)} \cdot \mathcal{S}^{22}_{(\text{PTC},p)\to(\text{diel},p+1)}, \tag{S23b}$$

$$\mathcal{S}^{21}_{(\text{diel},p)\to(\text{diel},p+1)} = \mathcal{S}^{21}_{(\text{diel},p)\to(\text{PTC},p)} + \mathcal{S}^{22}_{(\text{diel},p)\to(\text{PTC},p)} \cdot \chi_2 \cdot \mathcal{S}^{21}_{(\text{PTC},p)\to(\text{diel},p+1)} \cdot \mathcal{S}^{11}_{(\text{diel},p)\to(\text{PTC},p)}, \tag{S23c}$$

$$\mathcal{S}^{22}_{(\text{diel},p)\to(\text{diel},p+1)} = \mathcal{S}^{22}_{(\text{diel},p)\to(\text{PTC},p)} \cdot \chi_2 \cdot \mathcal{S}^{22}_{(\text{PTC},p)\to(\text{diel},p+1)}, \tag{S23d}$$

with $\chi_1 = \left(\mathbb{I} - \mathcal{S}^{12}_{(\text{diel},p)\to(\text{PTC},p)} \cdot \mathcal{S}^{21}_{(\text{PTC},p)\to(\text{diel},p+1)}\right)^{-1}$, $\chi_2 = \left(\mathbb{I} - \mathcal{S}^{21}_{(\text{PTC},p)\to(\text{diel},p+1)} \cdot \mathcal{S}^{12}_{(\text{diel},p)\to(\text{PTC},p)}\right)^{-1}$ and $\mathbb{I}$ denoting an identity matrix of dimension $2N+1$. Here, $\mathcal{S}^{ij}_{(\text{diel},p)\to(\text{diel},p+1)}$ denotes the $(i,j)$-th $(2N+1)$-dimensional block matrix of $\mathcal{S}_{(\text{diel},p)\to(\text{diel},p+1)}$ of dimension $2(2N+1)$. When considering the case of a cascade of $N$ units, we can obtain the scattering matrices $\mathcal{S}_{(\text{diel},1)\to(\text{PTC},1)}$, $\mathcal{S}_{(\text{PTC},1)\to(\text{diel},2)}$, $\mathcal{S}_{(\text{diel},2)\to(\text{PTC},2)}$, $\mathcal{S}_{(\text{PTC},2)\to(\text{diel},3)}$, $\mathcal{S}_{(\text{diel},3)\to(\text{PTC},3)}$, $\ldots$, $\mathcal{S}_{(\text{PTC},Nt-1)\to(\text{diel},Nt)}$, $\mathcal{S}_{(\text{diel},Nt)\to(\text{PTC},Nt)}$ at every interface. By successively cascading adjacent scattering matrices according to an approach similar to that of (S23), we can obtain $\mathcal{S}_{(\text{diel},1)\to(\text{diel},2)}$, $\mathcal{S}_{(\text{diel},1)\to(\text{PTC},2)}$, $\mathcal{S}_{(\text{diel},1)\to(\text{diel},3)}$, $\mathcal{S}_{(\text{diel},1)\to(\text{PTC},3)}$, $\ldots$, and finally the overall scattering matrix $\mathcal{S}_{(\text{diel},1)\to(\text{PTC},Nt)}$. The coefficients in the first dielectric layer $\boldsymbol{\tau}^{\text{diel}}_1$ and $\boldsymbol{r}^{\text{diel}}_1$, and the coefficients in the last PTC layer $\boldsymbol{\tau}^{\text{PTC}}_{Nt}$ and$\boldsymbol{r}^{\text{PTC}}_{Nt}$ can be related as

$$\begin{pmatrix} \boldsymbol{\tau}^{\text{PTC}}_{Nt} \\ \boldsymbol{r}^{\text{diel}}_1 \end{pmatrix} = \mathcal{S}_{(\text{diel},1)\to(\text{PTC},Nt)} \cdot \begin{pmatrix} \boldsymbol{\tau}^{\text{diel}}_1 \\ \boldsymbol{r}^{\text{PTC}}_{Nt} \end{pmatrix}. \tag{S24}$$

Often, the scattering matrix-cascading method is suitable when calculating the eigen-frequencies of the limited layers with the open boundary condition, as shown in FIG. S3. At the perfect electric conductor (PEC) boundaries when $z = z_0$ and $z = z_{Nt,2}$, we have $E^{\text{diel}}_{x,1}(z_0,t) = 0$ and $E^{\text{PTC}}_{x,Nt}(z_{Nt,2},t) = 0$, resulting in

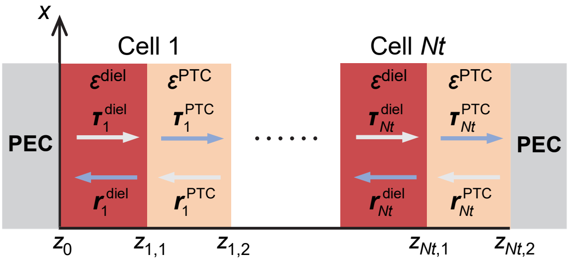


FIG. S3. Illustration of open boundary condition.

$$\begin{pmatrix} \boldsymbol{\phi}^{\text{diel}}_{1,2} & 0 \\ 0 & \Psi\boldsymbol{\phi}^{*\text{PTC}}_{Nt,2} \end{pmatrix} \begin{pmatrix} \boldsymbol{\tau}^{\text{diel}}_1 \\ \boldsymbol{r}^{\text{PTC}}_{Nt} \end{pmatrix} = \begin{pmatrix} 0 & -\boldsymbol{\phi}^{*\text{diel}}_{1,2} \\ -\Psi\boldsymbol{\phi}^{\text{PTC}}_{Nt,2} & 0 \end{pmatrix} \begin{pmatrix} \boldsymbol{\tau}^{\text{PTC}}_{Nt} \\ \boldsymbol{r}^{\text{diel}}_1 \end{pmatrix}. \tag{S25}$$

Finally, by incorporating (S25) with (S24), the eigen-frequencies $\omega$ can be solved according to the following characteristic equation:

$$g(\omega) = \det\left[\mathcal{S}_{(\text{diel},1)\to(\text{PTC},Nt)} + \begin{pmatrix} 0 & \boldsymbol{\phi}^{*\text{diel}}_{1,2} \\ \Psi\boldsymbol{\phi}^{\text{PTC}}_{Nt,2} & 0 \end{pmatrix}^{-1} \cdot \begin{pmatrix} \boldsymbol{\phi}^{\text{diel}}_{1,2} & 0 \\ 0 & \Psi\boldsymbol{\phi}^{*\text{PTC}}_{Nt,2} \end{pmatrix}\right] = 0. \tag{S26}$$

Although the scattering matrix method (SMM) has been widely utilized when calculating the total transmission and/or reflection coefficients owing to its numerical stability [S1, S2], it is not convenient when evaluating the band structure of the STMPCs. Next, we derive the details of transfer matrix method (TMM), which is feasible for STMPCs.

### D. Transfer matrix method

Unlike the SMM, the forward and backward waves in the same layer serve as input for the next layer within the TMM, as shown in FIG. S2 . The transfer equations at the boundaries $z = z_{p,1}$ and $z = z_{p,2}$ can be respectively as

$$\mathcal{T} \cdot \Phi^{\text{PTC}}_{p,1} \cdot \mathcal{C}^{\text{PTC}}_{p} = \mathcal{M} \cdot \Phi^{\text{diel}}_{p,1} \cdot \mathcal{C}^{\text{diel}}_{p}, \tag{S27a}$$

$$\mathcal{M} \cdot \Phi^{\text{diel}}_{p,2} \cdot \mathcal{C}^{\text{diel}}_{p+1} = \mathcal{T} \cdot \Phi^{\text{PTC}}_{p,2} \cdot \mathcal{C}^{\text{PTC}}_{p}, \tag{S27b}$$

where

$$\mathcal{T} = \begin{pmatrix} \Psi & 0 \\ 0 & \Psi\mathcal{Q} \end{pmatrix} \cdot \begin{pmatrix} \mathbb{I} & \mathbb{I} \\ \mathbb{I} & -\mathbb{I} \end{pmatrix}, \tag{S28a}$$

$$\mathcal{M} = \begin{pmatrix} \mathbb{I} & 0 \\ 0 & \mathcal{K} \end{pmatrix} \cdot \begin{pmatrix} \mathbb{I} & \mathbb{I} \\ \mathbb{I} & -\mathbb{I} \end{pmatrix}, \tag{S28b}$$

$$\Phi^{\text{PTC}}_{p,1(2)} = \text{diag}[\boldsymbol{\phi}^{\text{PTC}}_{p,1(2)}, \boldsymbol{\phi}^{*\text{PTC}}_{p,1(2)}], \tag{S28c}$$

$$\Phi^{\text{diel}}_{p,1(2)} = \text{diag}[\boldsymbol{\phi}^{\text{diel}}_{p,1(2)}, \boldsymbol{\phi}^{*\text{diel}}_{p,1(2)}], \tag{S28d}$$

$$\mathcal{C}^{\text{PTC}}_{p} = [\boldsymbol{\tau}^{\text{PTC}}_{p}, \boldsymbol{r}^{\text{PTC}}_{p}]^{\text{T}}, \tag{S28e}$$

$$\mathcal{C}^{\text{diel}}_{p} = [\boldsymbol{\tau}^{\text{diel}}_{p}, \boldsymbol{r}^{\text{diel}}_{p}]^{\text{T}} \tag{S28f}$$

with the phase matrices $\boldsymbol{\phi}$ being defined as

$$\boldsymbol{\phi}^{\text{PTC}}_{p,1(2)} = \text{diag}[e^{\text{i}q_1 z_{p,1(2)}}, \ldots, e^{\text{i}q_{N+1} z_{p,1(2)})}, \ldots, e^{\text{i}q_{2N+1} z_{p,1(2)}}], \tag{S29a}$$

$$\boldsymbol{\phi}^{\text{diel}}_{p,1(2)} = \text{diag}[e^{\text{i}k^{\text{diel}}_{-N} z_{p,1(2)}}, \ldots, e^{\text{i}k^{\text{diel}}_{0} z_{p,1(2)}}, \ldots, e^{\text{i}k^{\text{diel}}_{N} z_{p,1(2)}}]. \tag{S29b}$$

Therefore, we can obtain $\mathcal{C}^{\text{diel}}_{p+1} = (\mathcal{M} \cdot \Phi^{\text{diel}}_{p,2})^{-1} \cdot (\mathcal{T} \cdot \Phi^{\text{PTC}}_{p,2}) \cdot (\mathcal{T} \cdot \Phi^{\text{PTC}}_{p,1})^{-1} \cdot (\mathcal{M} \cdot \Phi^{\text{diel}}_{p,1}) \cdot \mathcal{C}^{\text{diel}}_{p}$, *i.e.*,

$$\mathcal{C}^{\text{diel}}_{p+1} = (\Phi^{\text{diel}}_{p,2})^{-1} \cdot (\mathcal{M}^{-1}\mathcal{T}) \cdot \left[\Phi^{\text{PTC}}_{p,2} (\Phi^{\text{PTC}}_{p,1})^{-1}\right] \cdot (\mathcal{T}^{-1}\mathcal{M}) \cdot \Phi^{\text{diel}}_{p,1} \cdot \mathcal{C}^{\text{diel}}_{p}. \tag{S30}$$

According to the Bloch theorem, electromagnetic waves at the interfaces $z = z_{p,1}$ and $z = z_{p+1,1}$ satisfy $E_x(z_{p+1,1}) = e^{\text{i}kd} E_x(z_{p,1})$ and $H_y(z_{p+1,1}) = e^{\text{i}kd} H_y(z_{p,1})$, repsectively, that is,

$$\Phi^{\text{diel}}_{p+1,1} \cdot \mathcal{C}^{\text{diel}}_{p+1} = e^{\text{i}kd} \Phi^{\text{diel}}_{p,1} \cdot \mathcal{C}^{\text{diel}}_{p}, \tag{S31}$$

where $k$ denotes the quasi-momentum. By combining (S31) with (S30), the dispersion relation of the STMPCs can be expressed as

$$f(k,\omega) = \det\left[\Phi^{\text{diel}}_{p+1,1} \cdot (\Phi^{\text{diel}}_{p,2})^{-1} \cdot (\mathcal{M}^{-1}\mathcal{T}) \cdot (\Phi^{\text{PTC}}_{p,2} (\Phi^{\text{PTC}}_{p,1})^{-1}) \cdot (\mathcal{T}^{-1}\mathcal{M}) - e^{\text{i}kd}\mathbb{I}\right] = 0. \tag{S32}$$

A more detailed form of (S32) reads

$$\begin{aligned} \det\Bigg[ & \begin{pmatrix} \boldsymbol{\phi}^{\text{diel}}_{d_\text{m}} & 0 \\ 0 & \boldsymbol{\phi}^{*\text{diel}}_{d_\text{m}} \end{pmatrix} \cdot \begin{pmatrix} \mathbb{I} & \mathbb{I} \\ \mathbb{I} & -\mathbb{I} \end{pmatrix} \cdot \begin{pmatrix} \Psi & 0 \\ 0 & \mathcal{K}^{-1}\Psi\mathcal{Q} \end{pmatrix} \cdot \begin{pmatrix} \mathbb{I} & \mathbb{I} \\ \mathbb{I} & -\mathbb{I} \end{pmatrix} \cdot \\ & \begin{pmatrix} \boldsymbol{\phi}^{\text{PTC}}_{d_\text{t}} & 0 \\ 0 & \boldsymbol{\phi}^{*\text{PTC}}_{d_\text{t}} \end{pmatrix} \cdot \begin{pmatrix} \mathbb{I} & \mathbb{I} \\ \mathbb{I} & -\mathbb{I} \end{pmatrix} \cdot \begin{pmatrix} \Psi^{-1} & 0 \\ 0 & \mathcal{Q}^{-1}\Psi^{-1}\mathcal{K} \end{pmatrix} \cdot \begin{pmatrix} \mathbb{I} & \mathbb{I} \\ \mathbb{I} & -\mathbb{I} \end{pmatrix} - 4e^{\text{i}kd} \cdot \begin{pmatrix} \mathbb{I} & 0 \\ 0 & \mathbb{I} \end{pmatrix} \Bigg] = 0, \end{aligned} \tag{S33}$$

where

$$\boldsymbol{\phi}^{\text{diel}}_{d_\text{m}} = \text{diag}[e^{\text{i}k^{\text{diel}}_{-N} d_\text{m}}, \ldots, e^{\text{i}k^{\text{diel}}_{0} d_\text{m}}, \ldots, e^{\text{i}k^{\text{diel}}_{N} d_\text{m}}], \tag{S34a}$$

$$\boldsymbol{\phi}^{\text{PTC}}_{d_\text{t}} = \text{diag}[e^{\text{i}q_1 d_\text{t}}, \ldots, e^{\text{i}q_{N+1} d_\text{t}}, \ldots, e^{\text{i}q_{2N+1} d_\text{t}}]. \tag{S34b}$$

Finally, one can obtain the band structure by working with (S32) or (S33).

## S2. DETAILED DISCUSSIONS ON THE PARAMETERS OF THE TRANSFORMED MATERIAL

Here, we present a strategy to obtain the exact form of the transformed material $\boldsymbol{G}$. Using the Fourier series expansion, we can obtain $\boldsymbol{B}^\dagger = \sum_p \boldsymbol{B}_p^\dagger e^{-\mathrm{i}p\Omega t}$ and $\psi^{\mathrm{L}} = \sum_m |\psi_m^{\mathrm{L}}\rangle = \sum_m \psi_m^{\mathrm{L}} e^{-\mathrm{i}m\Omega t}$, where $\Omega$ denotes the fundamental frequency. Likewise, the adjoint material $\boldsymbol{G}$ may also be expressed in terms of series as

$$\boldsymbol{G} = \sum_{q=-\infty}^{\infty}\sum_{m=-\infty}^{\infty} \boldsymbol{G}_{qm} e^{-\mathrm{i}(q-m)\Omega t}. \tag{S35}$$

where the component $\boldsymbol{G}_{qm}$ denotes the action on $\psi_m^{\mathrm{L}}$ which corresponds to the conversion of the $m$-th harmonic mode $|\psi_m^{\mathrm{L}}\rangle$ to the $q$-th harmonic mode $|\psi_q^{\mathrm{L}}\rangle$. Now, by virtue of the Cauchy product of series, the material transformation equation

$$(\mathrm{i}\partial_t + \omega^*)(\boldsymbol{G}\psi^{\mathrm{L}}) = \boldsymbol{B}^\dagger(\mathrm{i}\partial_t + \omega^*)\psi^{\mathrm{L}} \tag{S36}$$

can be reformulated as

$$\sum_{q=-\infty}^{\infty}\sum_{m=-\infty}^{\infty} [q\Omega + \omega^*]\boldsymbol{G}_{qm}\psi_m^{\mathrm{L}} e^{-\mathrm{i}q\Omega t} = \sum_{n=-\infty}^{\infty}\sum_{p=-\infty}^{\infty} (n\Omega + \omega^*)\boldsymbol{B}_p^\dagger \psi_n^{\mathrm{L}} e^{-\mathrm{i}(n+p)\Omega t}. \tag{S37}$$

By replacing $n+p$, $p$ by $p$, $p-n$, respectively, on the right-hand side, (S37) can be further expressed as

$$\sum_{m,q}(q\Omega + \omega^*)\boldsymbol{G}_{qm}\psi_m^{\mathrm{L}} e^{-\mathrm{i}q\Omega t} = \sum_{n,p}(n\Omega + \omega^*)\boldsymbol{B}_{p-n}^\dagger \psi_n^{\mathrm{L}} e^{-\mathrm{i}n\Omega t} \tag{S38}$$

Furthermore, by replacing $p$ by $q$ on the right-hand side, we obtain

$$\sum_{m,q}(q\Omega + \omega^*)\boldsymbol{G}_{qm}\psi_m^{\mathrm{L}} e^{-\mathrm{i}q\Omega t} = \sum_{n,q}(n\Omega + \omega^*)\boldsymbol{B}_{q-n}^\dagger \psi_n^{\mathrm{L}} e^{-\mathrm{i}q\Omega t}. \tag{S39}$$

Now, for each $q \in \mathbb{Z}$, we have

$$\sum_{m}(q\Omega + \omega^*)\boldsymbol{G}_{qm}\psi_m^{\mathrm{L}} = \sum_{n}(n\Omega + \omega^*)\boldsymbol{B}_{q-n}^\dagger \psi_n^{\mathrm{L}}. \tag{S40}$$

Truncating the integers $m,n,q \in [-N,N]$ in (S40), we can derive a sufficient solution for the adjoint material, which reads

$$\boldsymbol{G}_{qn} = (q\Omega + \omega^*)^{-1}\boldsymbol{B}_{q-n}^\dagger(n\Omega + \omega^*) \tag{S41}$$

for $q \in [-N,N]$ and $n \in [-N,N]$. Now, $\boldsymbol{G}$ can be reconstructed according to (S35) since $\boldsymbol{B}^\dagger$ can be easily obtained. For numerical calculations, $\boldsymbol{B}_{q-n}$ and $\boldsymbol{G}_{qm}$ are sufficient to construct transfer matrices or scattering matrices. By computing the right eigenstates of the adjoint system with the transformed material $\boldsymbol{G}$ using the TMM (see Supplemental Material, S1), subsequently one can derive the left eigenstates of the original system with the original material $\boldsymbol{B}$; furthermore, the biorthogonal Berry connection can be determined accordingly (see Supplemental Material, S3).

For the STMPCs discussed in the main text, the parameters of the transformed material can be obtained by

$$\boldsymbol{G}_{qn} = (q\Omega + \omega^*)^{-1}\boldsymbol{B}_{q-n}^\dagger(n\Omega + \omega^*). \tag{S42}$$

where the material sub-matrix $\boldsymbol{B}_{q-n}^\dagger$ comprise of the permittivity tensors $\boldsymbol{\varepsilon}_{q-n}$, permeability tensors $\boldsymbol{\mu}_{q-n}$, and magneto-electric coupling tensors $\boldsymbol{\xi}_{q-n}$ and $\boldsymbol{\zeta}_{q-n}$, that is,

$$\boldsymbol{B}_{q-n}^\dagger = \begin{pmatrix} \boldsymbol{\varepsilon}_{q-n} & \boldsymbol{\xi}_{q-n} \\ \boldsymbol{\zeta}_{q-n} & \boldsymbol{\mu}_{q-n} \end{pmatrix}. \tag{S43}$$

When $q=n$, we have $\boldsymbol{G}_{nn} = \boldsymbol{B}_0^\dagger$, indicating that the block matrices $\boldsymbol{G}_{nn} = \boldsymbol{B}_0^\dagger$ on the main diagonal of $\boldsymbol{G}$ remain invariant during the transformation. For time-invariant dielectric layers, we have $\boldsymbol{B}_{q-n}^\dagger = \delta_{q,n}\boldsymbol{B}_0^\dagger$ with $\delta_{q,n}$ being the Kronecker symbol, indicating that the transformed parameter matrix $\boldsymbol{G}$ only has sub-matrices $\boldsymbol{B}_0^\dagger$ on the main diagonal. Hence, the parameters for the normal dielectric layers remain invariant during the transformation.

For the temporally modulated layers, each of parameters $\boldsymbol{\varepsilon}_{q-n}$, $\boldsymbol{\mu}_{q-n}$, $\boldsymbol{\xi}_{q-n}$, $\boldsymbol{\zeta}_{q-n}$ needs to be transformed as

$$\boldsymbol{\varepsilon}_{q-n}' = (q\Omega + \omega^*)^{-1}\boldsymbol{\varepsilon}_{q-n}(n\Omega + \omega^*), \tag{S44a}$$

$$\boldsymbol{\mu}'_{q-n} = (q\Omega+\omega^*)^{-1}\boldsymbol{\mu}_{q-n}(n\Omega+\omega^*), \tag{S44b}$$

$$\boldsymbol{\xi}'_{q-n} = (q\Omega+\omega^*)^{-1}\boldsymbol{\xi}_{q-n}(n\Omega+\omega^*), \tag{S44c}$$

$$\boldsymbol{\zeta}'_{q-n} = (q\Omega+\omega^*)^{-1}\boldsymbol{\zeta}_{q-n}(n\Omega+\omega^*), \tag{S44d}$$

which form $\boldsymbol{G}_{qn}$ as

$$\boldsymbol{G}_{qn} = \begin{pmatrix} \boldsymbol{\varepsilon}'_{q-n} & \boldsymbol{\xi}'_{q-n} \\ \boldsymbol{\zeta}'_{q-n} & \boldsymbol{\mu}'_{q-n} \end{pmatrix}. \tag{S45}$$

In the main text, we consider the scenario when only the permittivity tensor $\boldsymbol{\varepsilon}$ is temporal modulated, which means $\boldsymbol{\mu}_0 = \boldsymbol{\xi}_0 = \boldsymbol{\zeta}_0 \neq \mathbf{0}$ in the Fourier series expansion. Consequently, for the transformation described in (S42), the time-invariant parameters remain the same, *i.e.*, $\boldsymbol{\mu}'_{m,n} = \delta_{q,n}\boldsymbol{\mu}_0$, $\boldsymbol{\xi}'_{m,n} = \delta_{q,n}\boldsymbol{\xi}_0$, and $\boldsymbol{\zeta}'_{m,n} = \delta_{q,n}\boldsymbol{\zeta}_0$; and the time-varying permittivity after transformation is $\boldsymbol{\varepsilon}'_{m,n} = (q\Omega+\omega^*)^{-1}\boldsymbol{\varepsilon}_{q-n}(n\Omega+\omega^*)$. We note that the band structure $(\omega,k)$ of the original system should be worked out before the transformation (S44) to obtain the material parameters of the adjoint system. For the adjoint system, the TMM introduced in Supplemental Material, S1 can be used to calculate the field distribution of the adjoint system with transformed parameters $\boldsymbol{\varepsilon}', \boldsymbol{\mu}', \boldsymbol{\xi}', \boldsymbol{\zeta}'$. Specifically, for the STMPCs discussed in the main text, one can simply substitute the components of the permittivity matrix $\mathcal{E}$ in (S8) with $\boldsymbol{\varepsilon}'_{q,n}$.

## S3. CALCULATING THE ZAK PHASE WITHIN WILLSON LOOP METHOD

In order to calculate the Zak phase, the field distribution is required within one spatial period. Without loss of generality, we assume that the origin $z = 0$ is located in the center of a PTC layer and that the entire structure is symmetric with respect to the origin, as shown in FIG. S4 .

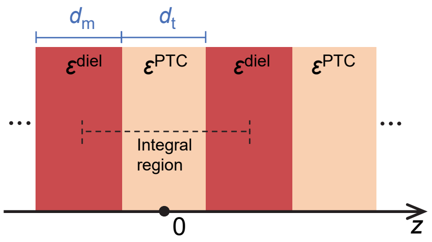


FIG. S4. Illustration for Zak phase calculation.

For a one-dimensional Hermition system, the Zak phase can be defined as [S3]

$$\theta_i = \int_{\partial B} \langle \psi_{i,k} \,|\, \partial_k \psi_{i,k} \rangle \,\mathrm{d}k, \tag{S46}$$

where the integral interval $\partial B$ is the first Brillouin region and $|\psi_{i,k}\rangle$ is the Bloch component of the electromagnetic eigenmode corresponding to the band $i$. However, for the non-Hermition STMPCs, (S46) needs to be modified to

$$\theta_i = \int_{\partial B} \langle \psi^{\mathrm{L}}_{i,k} \,|\, \partial_k \psi^{\mathrm{R}}_{i,k} \rangle \,\mathrm{d}k, \tag{S47}$$

where superscripts 'L' and 'R' denote the left and right eigenmodes, respectively. According to Eq. (1) in the main text, the bi-orthogonal Berry connection $\mathcal{A}_k$ in a photonic crystal reads

$$\mathcal{A}_k = \langle \psi^{\mathrm{L}}_{i,k} \,|\, \partial_k \psi^{\mathrm{R}}_{i,k} \rangle = \int_{-d/2}^{d/2} [\psi^{\mathrm{L}}_{i,k}(z)]^* \mathcal{B}(z) \partial_k \psi^{\mathrm{R}}_{i,k}(z) \mathrm{d}z, \tag{S48}$$

where eigenmodes $\psi^{\mathrm{L}}_{i,k}(z)$ and $\psi^{\mathrm{R}}_{i,k}(z)$ are respectively defined as

$$\psi^{\mathrm{L}}_{i,k}(z) = \left[E^{\mathrm{L}}_{x,k,-N}(z), H^{\mathrm{L}}_{y,k,-N}(z), \ldots, E^{\mathrm{L}}_{x,k,N}(z), H^{\mathrm{L}}_{y,k,N}(z)\right] e^{-\mathrm{i}kz}, \tag{S49a}$$

$$\psi^{\mathrm{R}}_{i,k}(z) = \left[E^{\mathrm{R}}_{x,k,-N}(z), H^{\mathrm{R}}_{y,k,-N}(z), \ldots, E^{\mathrm{R}}_{x,k,N}(z), H^{\mathrm{R}}_{y,k,N}(z)\right] e^{-\mathrm{i}kz}. \tag{S49b}$$

where $E^{\mathrm{L/R}}_{x,k,n}(z)$ and $H^{\mathrm{L/R}}_{y,k,n}(z)$ denote the $n$-th electric and magnetic harmonics with quasi-momentum $k$, respectively; the superscripts 'L' and 'R' for the fields indicate the left eigenmodes derived from the adjoint system and the right eigenmodes derived from the original system, respectively. Note that time harmonics are truncated by $N$-th order.

In general, it is difficult to obtain the explicit expression of $\partial_k \psi^{\mathrm{L/R}}_{i,k}$, and the discrete Wilson-loop approach is adopted [S4, S5]. Thus, we have

$$\theta_i = -\Im\left\{\ln\left[\prod_{l=1}^{L}\left\langle \psi^{\mathrm{L}}_{i,k_l} \middle| \psi^{\mathrm{R}}_{i,k_{l+1}}\right\rangle\right]\right\}, \tag{S50}$$

where $\Im[\bullet]$ denotes the imaginary part. Here, the integral interval is partitioned into $L$ segments, namely $[k_l, k_{l+1}]$. Since temporal periodicity yields momentum band gaps and results in entangled bands, the (discrete) Berry connection in (S50) must be corrected according to the determinant of overlap matrices $\mathcal{U}(k_l, k_{l+1})$ with elements $\mathcal{U}_{i,j} = \left\langle \psi^{\mathrm{L}}_{i,k_l} \middle| \psi^{\mathrm{R}}_{j,k_{l+1}}\right\rangle$ [S4, S5]. Now, the Zak phase of the entangled bands reads

$$\theta = -\Im\left\{\ln\left[\det\left(\prod_{l=1}^{L}\mathcal{U}(k_l, k_{l+1})\right)\right]\right\}. \tag{S51}$$

## S4. BENCHMARK

From the aspects of the governing equations (i.e., Eq. (1) and Eq. (4) in the main text), the original system and adjoint system may theoretically have similar band structures, which have conjugate quasi-frequencies $\omega$. To demonstrate the effectiveness of the transformed material method, we consider an example of a one-dimensional STMPC of spatial period $\Lambda$, which consists of dielectrics $\varepsilon_d = 2$ and PTCs characterized by $\varepsilon_t(t) = 6(1+\alpha\sin\Omega t)$ arranged in a spatially periodic manner, where $\Omega$ represents the frequency of the temporal modulation. Here, we adopt $\Omega = 0.2\omega_0$ with $\omega_0 = c_0/(2\pi\Lambda)$; in addition, non-magnetic materials are considered for simplicity, *i.e.*, $\mu = 1$. The thicknesses of the PTC and the dielectric in a unit cell read $l_{\mathrm{t}} = \eta\Lambda$ and $l_{\mathrm{d}} = (1-\eta)\Lambda$, respectively, where $\eta$ denotes the filling ratio. The coordinate origin $z = 0$ is located in the center of a PTC layer. When calculating the band structure of the adjoint system, according to the transformation strategy in (S42), only the permittivity $\varepsilon_{\mathrm{t}}$ needs to be modified to $\varepsilon'_{\mathrm{t}}$ (see Supplemental Material, S2), and other geometric and material characteristics remain unchanged. Note that the time harmonics are truncated to $N_t = 1$ for the temporally sinusoidal modulation.

FIG. S5 exhibits the band structures of both the original and the corresponding adjoint systems for different filling ratios $\eta$ of 0.1, 0.25, 0.4 and 0.6 (from left to right), which are obtained using the TMM. The top and bottom panels exhibit the real and imaginary components of the band structures, respectively, for which the quasi-frequencies $\omega$ and quasi-momentums $k$ normalized by $\omega_0$ and $k_d = 2\pi/\Lambda$, respectively. It is validated that the system with transformed material is the adjoint system of the original one. Unlike exclusive space-modulated PCs, both frequency gaps and momentum band gaps exist. The momentum band gaps are located at half the temporal modulation frequency $\Omega/2$, which is not affected by the filling ratio $\eta$. As the fill ratio $\eta$ increases, the separation distance between the momentum gaps increases, as well as the imaginary components of quasi-frequencies within the gap. Therefore, by adjusting the filling ratio $\eta$, it is possible to manipulate the quasi-momentum $k$ and the amplification intensity of the enhanced mode located within the momentum band gaps to some extent.

## S5. BAND INVERSION BETWEEN DEGENERATE BANDS AND ISOLATED BANDS

The band inversion phenomenon also occurs between isolated bands and degenerate bands. FIG. S6**(a)** and FIG. S6**(b)** show the entangled bands 2–5 and the isolated band 6 when the filling ratios read $\eta_1 = 0.20$ and $\eta_2 = 0.24$, respectively. For the isolated band 6 depicted in FIG. S6**(a)**, the eigenstates at the edge and center of the band show different symmetry characteristics, leading to a non-trivial Zak phase of $\theta_6 = 1$. For the entangled bands 2–5, the total Zak phase reads $\theta_{2-5} = 1$, which can be calculated using the TMM with the transformed material. In FIG. S6**(b)**, the isolated band 6 has a Zak phase of $\theta_6 = 0$, and the entangled bands 2–5 have a total Zak phase $\theta_{2-5} = 0$. Due to the presence of the degenerate point, as marked 's' in FIG. S6**(a)** and FIG. S6**(b)**, the field distribution of the eigenstates at this point cannot be classified based on the condition of $|E_{x,k,n}(z=0)| = 0$. Hence, the total Zak phase of the entangled bands cannot be determined by correlation of the symmetry characteristics of the field distribution between the eigenstates at the band edge and center. Inversion of the band at the boundary of bands 5 and 6, as seen in FIG. S6**(c-f)**, may still result in a transition of the Zak phase for both isolated and entangled bands. The results imply that the transition of the Zak phase of the STMPCs may be explained by the band inversion proposed by Zak [S3], regardless of whether the eigenstate resides within isolated or entangled bands.

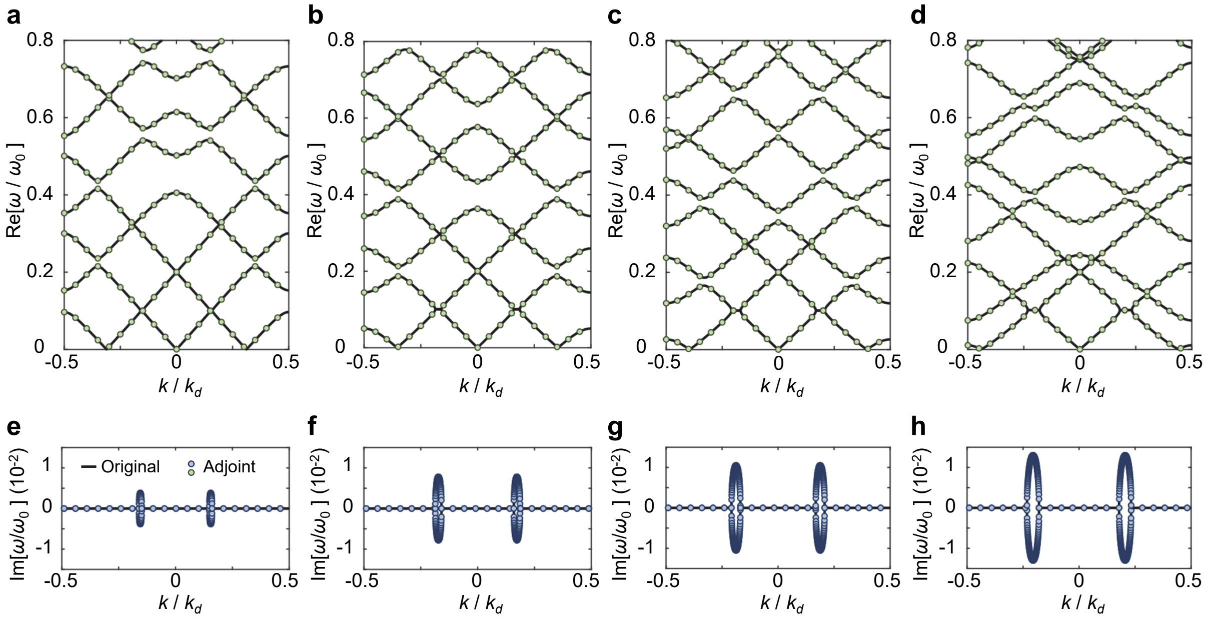


FIG. S5. **Complex band structures for STMPCs with different filling ratios $\eta$. a–d**, Real components of the quasi-frequencies $\omega$ when $\eta$ reads 0.1, 0.25, 0.4, and 0.6, respectively. **e–h**, Imaginary components of quasi-frequencies $\omega$ at correspond to **a–d**, respectively. Solid lines and dots represent the band structures of the original and adjoint systems, respectively. Green and blue dots indicate the real and imaginary components of quasi-frequencies $\omega$, respectively.

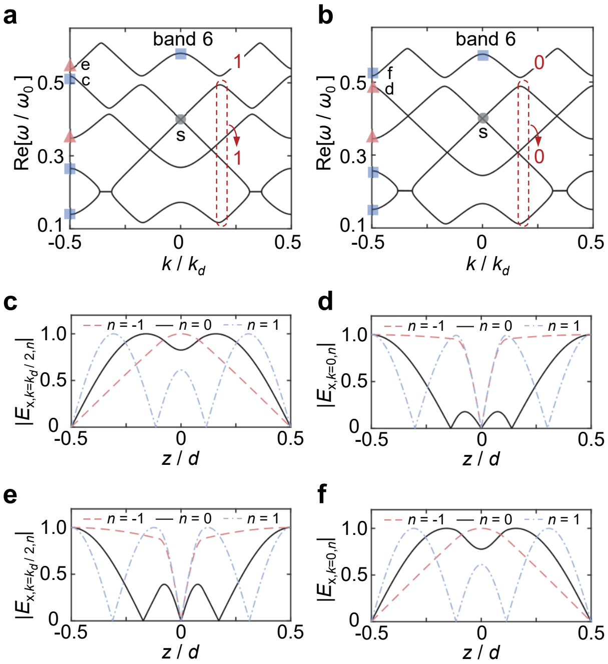


FIG. S6. **Band inversion between degenerate bands and isolated bands.** Band structures of bands $2-6$ when the filling ratio reads (**a**) $\eta = 0.20$ and (**b**) $\eta = 0.24$, respectively. Numbers on the bands labels the Zak phases. The triangular and cubic markers signify the eigenstates with distinct symmetries at the band edges. (**c**–**f**) The distribution of the normalized electric field $|E_{x,k,n}|$ corresponding respectively to the eigenstates labeled ‘c–f’ in (**a**) and (**b**). The dashed, solid, and dotted lines indicate the harmonics with the order of $n = -1, 0, 1$, respectively.

[S1] T. Dong, Y. Shi, L. Lu, F. Chen, X. Ma, and R. Mittra, Optical response of cylindrical multilayers in the context of hydrodynamic convection-diffusion model, J. Appl. Phys. **120**, 123102 (2016).

[S2] X. Gao, X. Zhao, R. Huang, S. Ma, X. Ma, and T. Dong, Analysis and design of transition radiation in layered uniaxial crystals using tandem neural networks, J. Opt. Soc. Am. B **40**, 645 (2023).

[S3] J. Zak, Berry's phase for energy bands in solids, Phys. Rev. Lett. **62**, 2747 (1989).

[S4] M. Blanco de Paz, C. Devescovi, G. Giedke, J. J. Saenz, M. G. Vergniory, B. Bradlyn, D. Bercioux, and A. García-Etxarri, Tutorial: computing topological invariants in 2D photonic crystals, Adv. Quantum Technol. **3**, 1900117 (2020).

[S5] K. Ding, Z. Zhang, and C. T. Chan, Coalescence of exceptional points and phase diagrams for one-dimensional $\mathscr{PT}$-symmetric photonic crystals, Phys. Rev. B **92**, 235310 (2015).
